# Supplementary material for: Metabolic fluxes and value production
Source: arXiv:1404.5072 source file (2022-10-04)
Supplement: Supplementary file 1 [file sec_supplement_flux_analysis_cba.tex]

\co{WO? WEG? 
  \includegraphics[width=4.cm]{\psfilesfluxes/cba_yeast_ccm_futile_cycles_hist_futile_cycles.eps}

  Size distribution of elementary {\nonbeneficial} submodes. Typical
  sizes (numbers of active reactions) range between 20 and 40.}

\co{WO? 

  refers to Fig 5
  
  \myparagraph{Economic potentials and degradation costs} \co{discuss
  case of negative economic potentials; weiter unten: what's the direction of the
  value flow?} Interestingly, the economic potential can also tell us
about  enzyme investments downstream of the
metabolite: the economic potential of our metabolite X can also we
written as $w_{\rm X} = w_{\rm P} - \frac{z_{x \rightarrow p}}{v}$,
the economic potential of end product P minus the sum of enzyme
investments needed to convert X into P, divided by the flux.  \co{if
  the substrate was a ``free gift'', the economic potentials are given
  by the enzyme investments divided by the flux.} For example, we can
think of a toxic metabolite X, which needs to be converted into an
extracellular waste product (with a zero value). The economic
potential of X must be given by the total {\enzymeinvestment} of the
detoxification pathway (including export proteins), divided by the
detoxification flux, and with a minus sign. \co{was lernen wir?}
\co{however, negatives potential heisst nicht direkt gift} \co{auch
  auf simple ccm beispiel in cba II verweisen?}  \co{2. general
  inference of economic values and {\valueflow}s // reference to
  abchnitt in CBA I zu inference of economic potentials from variation
  conditions // hier nur schematisches bild mit wachsenden pfeilen?
  oder lieber nur in CBA lagrange?}
}

\section{How metabolic fluxes are shaped by enzyme economy}
\label{sec:potentialsinnetworks}

\co{allgemein $\zcostgeneric$  in SI verwenden}

\subsection{The usage of enzymes or pathways}

Under what conditions should different enzymes or pathways be used by
a cell?  In an optimal state, the {\fluxvalue} of an active
enzymatic reaction must be balanced with the {\fluxburden}, i.e.~the
{{\enzymeinvestment}} per flux. This means, first, if two reactions (or
pathways) have the same overall stoichiometry, only one of them can be
active -- unless the {\fluxburden}s are identical, which (given the
different kinetics) is highly unlikely\footnote{In reality, the flux
  {\burden}s may still be quite similar, and so use both enzymes
  together will almost be optimal.} Second, the maximal catalytic rate
of an enzyme defines a lower bound on the {\fluxburden}. For an
enzyme to be active, its {\fluxvalue} must exceed than this minimal
{\fluxburden}, and a similar rule can be given for entire
pathways. Let us see this  in detail

\myparagraph{A balance equation for linear pathways} In metabolic
models, a linear metabolic pathway can described, effectively as a
single reaction.  For a consistent economic theory, it is therefore,
important that economic balances for reactions and pathways have the
same form. In fact, we can easily derive a single pathway balance
equation between the total {\enzymeinvestment} and the total flux benefit.
With a pathway flux $v_{\rm L}$ (identical for all reactions; but
different flux stoichiometries can be takein into account), the
balance equation Eq.~(\ref{eq:gedankenexpsum}) can be written as
\begin{eqnarray}
 \label{eq:gedankenexpsum2}
 \left[\sum_{l \in L} \Deltar \wintl + \sum_{l \in L} \bvdirl \right]
v_{\rm L} = h_{u,L}\,\ul,
\end{eqnarray}
with the total pathway enzyme level $\ul=\sum_{l \in L} \,\ul$ and
apparent pathway cost
$h_{\rm u,L} = (\sum_{l} \ul\, \hul)/(\sum_{l} \ul)$.  \co{hier fehlt
  noch erklaereung von bvL. lieber die einfache formel betonen}
Eq.~(\ref{eq:gedankenexpsum2}), written as
$\Deltar w_{\rm L}\,v_{\rm L} = h_{\rm \u_L}\,\u_{\rm L}$, resembles
the balance equation for single reactions.  \co{also define effective
  ``pathway flux burden''}

\myparagraph{Lower bound on the  {\myvalue}}
\label{sec:usageofpathways} 
In a kinetic model, each enzyme has a maximal activity $k^{\rm cat}$
and a minimal {\price} $\hulmin$ (the cost per amount of enzyme at
small expression levels). The ratio $\hulmin/k^{\rm cat}$ defines a
lower bound on the {\fluxburden} \cite{nfbd:16}.  If the flux
{\myvalue} of the reaction is lower, the reaction must be inactive. To see this, we consider
the  {\fluxbenefitbalance}
(\ref{eq:reactionbalanceeq}) in the form\footnote{Here we assume
  (without loss of generality) that  flux and {\fluxburden}
  $\hvl$ are positive, and consider the $\kcat$ value in forward
  direction.}
\begin{eqnarray}
 \label{eq:forceequation}
  \Deltar \wtotl + \bvdirl = \frac{\hul} {v_{l}/\ul} = \hvl.
\end{eqnarray}
The enzyme {\price} $\hul$ is bounded from below by some lower value
$\hulmin$, and the catalytic rate $v_{l}/\ul$ is always lower than the
catalytic constant $k^{\rm cat} = (v_{l}/\ul)^{\rm max}$ (for the flux
direction chosen). Therefore, the ratio in
Eq.~(\ref{eq:forceequation}) will always be larger than
$\hvlmin = \hulmin / k^{\rm cat}$, which defines a lower bound on the
{\fluxburden}\footnote{To calculate the {\fluxburden} $\hvl$, we may
  estimate $\ul/v_{l}$ from measured proteome and flux data, while
  {{\enzymeprice}}s $\hul$ can be estimated from enzyme chain lengths,
  catalytic constants, and life times \cite{horh:11} (see SI
  \ref{sec:potentaislfromenzymepar}) \cite{szad:10}.\coout{Values for
    a rough numerical estimate are an effective lifetime of 30 minutes
    (for growing \emph{E.~coli} cells)} Of course, $k^{\rm cat}$ is
  only an upper bound on $v_{l}/\ul$; for a closer approximation, we
  may account for reversibility and thermodynamic forces
  \cite{nflb:13}. A further correction method for $\hvl$, assuming an
  optimal state, is described in section
  \ref{sec:SIAlgConstraintFluxBurden}. Finally, we may also put upper
  bounds on the {\fluxvalue} from estimates on the maximal
  {{\enzymeprice}} and on estimated minimal enzyme
  efficiencies.}. Note that the bound is a lower approximation only:
even at higher {\fluxvalue}s, the reaction may stay inactive. A
similar argument holds also for pathways instead of reactions. In an
unbranched pathway with a production objective and with lower
{{\enzymeinvestment}}s $\hulmin$, we can sum over the {\fluxbenefitbalance}s
and obtain the pathway balance
\begin{eqnarray}
\label{eq:criticalbenefit}
\Deltar w_{\rm L} = \sum_{l \in L} \frac{\hul\,\ul}{v_{l}} \ge \sum_{l \in L} \frac{\hulmin}{k^{\rm cat}_{l}}.
\end{eqnarray}
If the flux
{\myvalue} $\Deltar w_{\rm L}$ is below this bound, the pathway flux
cannot be economical.

\myparagraph{Choices between enzymes or
  pathways} \label{sec:isoenzymesandisopathways}
Isoenzymes are enzymes that catalyse the same reaction and share the
same {\fluxvalue}.  \coout{WEG? {\myvalue}
  $\gvtot = \Deltar \wint + \bvtot$. By taking the ratio of both flux
  benefit balances, we obtain
\begin{eqnarray}
 \label{isoenzymes1}
 \frac{(\Deltar w+z_{\rm v})\,v_{1} }{(\Deltar w+z_{\rm v})\,v_{2} } = \frac{\hminus_{u_{1}}\,u_{1}}{h^{\rm u}_{2}\,u_{2}} \qquad 
\Rightarrow \qquad \frac{h^{\rm u}_{1}\,u_{1}}{v_{1}} = \frac{h^{\rm u}_{2}\,u_{2}}{v_{2}} \qquad \Rightarrow \qquad {\hvs}_{1} = {\hvs}_{2}.
\end{eqnarray}
} Therefore, if two isoenzymes are simultaneously active in an optimal
state, their {\fluxburden}s (i.e.~{{\enzymeinvestment}}s per flux) must be
equal. If we pick a model (with randomly chosen kinetic constants) and
optimise its enzyme levels, it is highly unlikely that isoenzymes will
satisfy such an equality (unless they are physically identical).  Only
one the enzymes will be expressed, the one with the lower {\price}.
Like for single reactions, the {\fluxvalue} can also be used to
predict the choice between pathways.  In a pathway L, we define the
total enzyme level $\u_{L} = \sum_l \,\ul$ and the apparent
{\enzymeprice} $h_{u_L} = \frac{\sum_l \hul\,\ul}{\sum_l \ul}$; the
total {\enzymeinvestment} can therefore be written as
$y_L = \sum_l \zcostgenerics_{l} = h_{u_L}\,\u_{L}$.  With the representative
pathway flux $v_L$, we then define the pathway {\fluxburden}
$a_{v_L} = \frac{y_L}{v_L} = \frac{h_{u_L}\,\ul}{v_L}$, the total
enzyme cost per unit flux \cite{bnlm:10}.  If two pathways show the
same net flux stoichiometries, they are called
\emph{isopathways}. \co{The fluxes $v_{L}$ must be comparable between
  pathways, that is, pathways with equal fluxes $v_{L_{1}}=v_{L_{2}}$
  must show the same net conversion.} If the metabolic objective does
not depend on concentrations or fluxes inside the pathways, both
isopathways have the same {\fluxvalue}. To be simultaneously active,
they need to to satisfy
\begin{eqnarray}
 \label{isoenzymes2}
 \frac{v_{1}}{v_{2}} = \frac{\sum_{l \in 1} \hul\, \ul} {\sum_{l \in 2} \hul\, \ul} \qquad 
 \Rightarrow \qquad \frac{v_{1}/u_{1}^{\rm tot}}{h^{\rm u,tot}_{1}} = \frac{v_{2}/u^{\rm tot}_{2}}{h^{\rm u,tot}_{2}}
 \qquad \Rightarrow \qquad {\hvs^{\rm tot}}_{1} = {\hvs^{\rm tot}}_{2}
\end{eqnarray}
where $u^{\rm tot}_{L}$ is the total protein level in pathway $L$,
exactly the same {\fluxburden}.  However in a given kinetic model, it
is very unlikely that two isopathways satisfy this condition just by
chance, unless they are fully identical. \co{Thus, one of them will
  have a lower {\price} and will be preferred.}

\subsection{How to compute  economic potentials from fluxes and flux
  {\gain}s}
\label{sec:SIscalingProperties}

\co{mention proportional scaling of potential differences in
  unbranched chain?}  If fluxes or metabolic objectives in a pathway
are changing, the economic potentials will be changing, too.  The
metabolic objective of a pathway is reflected by the {\fluxgain}s
and, equivalently, by the economic potentials at the pathway
boundaries.  If a pathway is perturbed, the metabolic state changes,
and the precise changes depend on all kinetic details. To obtain rules
of thumb for the changing economic potentials, we consider an
approximation. \co{According to Eq.~(\ref{eq:balancedinvestments6}),
  the internal economic potentials depend linearly on external
  economic potentials and on direct {\fluxvalue}s.}  If economic
potentials are computed with heuristic assumptions as explained in
section \ref{sec:princdistribinvestment}, then given the pathway
fluxes $\vv$ and {\fluxgain}s $\bvtot$ (assuming uniform
{{\enzymeinvestment}}s and using Eq.~(\ref{eq:balancedinvestments4Opt})), or
given the fluxes $\vv$ and (approximate) {{\enzymeinvestment}}s
${\hudot}^{\rm data}$ (using Eq.~(\ref{eq:balancedinvestments6})), the
internal economic potentials can be computed from the external
economic potentials. Assuming either given or uniform
{{\enzymeinvestment}}s, we can determine the internal economic potentials as
a function $\wint(\vv,\wext)$.  This formula shows how perturbations
of fluxes $\vv$ or {\fluxgain}s $\bvtotweight$ affect the internal
economic potentials. For example, if we scale the external variables
($\vv$ and $\wext$) by a factor $\xi$, the changes in the internal
potentials follow from simple scaling considerations.  \co{diskutiere
  verschiedene skalierungsmoeglichkeiten: nochmal klarer machen, was
  bei princ of fixed {{\enzymeprice}}s los ist; hat flussskalierung
  einen einfluss auf minimal {\fluxvalue} constraint?}  \co{In
  addition, we need to consider the constraint S29?? and whether this
  constraint can still be satisfied after our perturbation.}
According to Eqs (\ref{eq:balancedinvestments3}) and
(\ref{eq:balancedinvestments6}), the economic potentials $\winti$
scale proportionally with the {\fluxgain}s $\bvtot$, but are not
affected by flux scaling. The constraint
Eq.~(\ref{eq:balancedinvestments4}) is affected by a scaling
$\wint \rightarrow \xi\,\wint, \bvtot\rightarrow \xi\,\bvtot$, and
also by a scaling $\vv \rightarrow \xi\,\vv$. However, it remains
unchanged under a simultaneous inverse scaling
$\wint \rightarrow \xi\,\wint, \bvtot\rightarrow \xi\,\bvtot, \vv
\rightarrow \frac{1}{\xi}\,\vv$.  Taken together, a flux increase (at
constant {\fluxgain}s $\bvtot$) leaves all internal economic
potentials unchanged, while the {{\enzymeinvestment}}s increase
proportionally. In contrast, an increase of the flux gains $\bvtot$
(at a constant flux) makes both $\wint$ and the {{\enzymeinvestment}}s
increase proportionally. If we \emph{decrease} the flux or flux
{\gain}, the {\enzymeinvestment}s decrease until the solution hits
a constraint; in this case, the pathway flux is switched off,
even though the \todo{desired flux or {\fluxgain}} was still
positive!  \co{The same conclusions holds both for the principles of
  uniform cost, known cost, uniform {{\enzymeprice}}s, and known
  {{\enzymeprice}}s.}  \co{They also remain valid if we consider the
  entire metabolic network instead of a single pathway.}  From these
scaling relationships, we can also obtain sum rules similar to the
theorems of Metabolic Control Theory (see the derivations in
\cite{lieb:18lagrange}). \co{die summenregeln als formeln angeben}

\subsection{Should cells use combined metabolic strategies?}  
\label{sec:SIcombinationOrAlternative}

\co{interessant: der abschnitt liefert eine direkte verbindung
  zwischen metabolic economic und FCM; vieleicht ausdruecklich darauf
  eingehen?}  \co{textteile von hier in den artikel schieben (hinter
  ``Isoenzymes and isopathways'')? teilweise nach artikel, teilweise
  hier diskutieren, welche rechenmethoden tatsaechlich verwendet
  werden sollen} \co{move some parts to other articles?}  \co{hier
  roten faden klarkriegen. realitaet; formalismus; praktische
  vorgehensweise beim samplen?}

\myparagraph{\ \\Pure and combined strategies} A cell may accomplish
the same production task by different pathways (e.g.~it may use
fermentation or respiration to produce ATP at a given rate). Moreover,
these pathways may be used separately or in combination, i.e.~by a
linear supposition of pathway fluxes. Also isoenzymes could either be
used exclusively or in combination. In reality, often one pathway is
used at a time: for example, when bacteria grow on glucose, they often
repress the uptake of other carbon sources, even if these carbon
sources are available in the growth medium\footnote{The co-utilisation
  of glucose and malate in \emph{B.~subtilis} is a known exception.}.
\co{below: consider the case in which two pathways provide exactly the
  same net consumption and production (except for fitness-neutral
  differences, e.g.~usage of different ``cost-free'' nutrients.}  In
VBA this leads to the question: given our polytope of
economical {\flow}s (with pure pathway strategies on the boundaries,
and combined strategies inside the polytope), should we assume that
real metabolic {\flow}s can be anywhere in the polytope, or should we
rather assume that real {\flow}s must be sparse, and thus on polytope
vertices?  In the first case, it would make sense to sample solutions
from the entire polytope, whereas in the second case, we should pick
solutions only among polytope vertices.  Interestingly, this is also
what is most likely to happen in FCM (or in FBA with a minimal
weighted sum of fluxes), where due to the concave or linear flux cost
functions, the solutions are likely to lie on the boundary\footnote{If
  we consider alternative pathways in linear FCM, one of the pathways
  will be selected depending on the flux cost weights in the two
  pathways. Only if the two alternative pathways are completely
  identical (including the flux costs), a superposition of the two
  pathways is also allowed. However, if the flux cost weights were
  chosen at random, this case occurs with zero probability.}.
\co{mention relation to EFMs, cite EFM-FCM} Finally, we may also
envisage a third possibility: cells might combine as many strategies
as possible, and realise a very non-sparse flux distribution in the
centre of the polytope.  So, in Figure \ref{fig:fbacomparison2}, for
example, will the {\flow} shown by cells be located in the entire blue
triangle, on the dark blue edges, or in the triangle center?

\myparagraph{Arguments for pure strategies} The idea that
metabolic flux distributions should be sparse and that alternative
pathways should not be used in combination is supported by several
arguments. First, in flux cost minimisation the enzymatic flux cost is
a concave function on the flux polytope, so enzyme-optimal {\flow}s will
be located on vertices of the (benefit-restricted) flux polytope
\cite{wpht:14,murs:14}.  \co{lieber: samplen?  wenn optimum gewuenscht
  wird, In practice, lieber sparse!}  Exceptions can only occur if two
enzymes or pathways show exactly the same kinetics and cost functions
\cite{lieb:18fcm}.  Kinetic models in enzyme-optimal states lead to
the same conclusion: if alternative pathways are used simultaneously,
they are subject to the same economic potential difference, so they
must show the same enzyme cost. If we sample kinetic models (by
randomly assigning kinetic constants) and compute their enzyme-optimal
flows, it is very unlikely that alternative pathways will have exactly
the same flux costs.  According to these arguments, pathways should
not be combined, and isoenzymes and isopathways should be used
alternatively rather than in combination.

\myparagraph{Arguments for combined strategies} However, there are
also arguments for using combined {\flow}s. The most striking argument is
that such modes are observed in cells \co{ueberlagerung von el modes.
  zb warburgeffekt} How can we obtain combined strategies in models?
First, a superposition of basic {\flow}s may be enforced by constraints
(e.g.~when the maximal capacity of respiration is reached due to
crowding of respiratory chain complexes on cell membranes, additional
overflow may be required.  Second, there might be optimality reasons
(analogous to constraints) for adjusting the cell state in such a way
that isoenzymes show identical flux burdens. \co{compare to
  self-organised criticality} Third, some side objectives may be more
important than strict cost optimality. For example, nutrient
transporters with binding affinities are often expressed
simultaneously. This contradicts the idea of strict cost minimisation,
but it may provide an advantage when cells need to anticipate possible
changes in their environment (changing concentrations of the
nutrient). Even if a combined strategy is sub-optimal, the cost
disadvantage may not be large.  There are many such cases of
preemptive protein expression. \co{consider ``free'' benefit, similar
  to ``free energy in thermodynamics''; discuss this in FCM, cite it
  here} In this case, it would be unrealistic to expect that only the
nominally best state (with sparse fluxes) is actually reached. So the
actual question would be: if a ``pure'' strategy is better than
combined strategies, how big is the actual fitness difference?

\myparagraph{Consequences for flux sampling} This question -- whether
cells should use sparse or combined fluxes -- is important for flux
prediction by sampling.  If we sample parameter variants of a kinetic
model and compute the enzyme-optimal states, we will \emph{only}
obtain {\flow}s that are polytope vertices, just like in FCM.  However,
if we sample {\flow}s uniformly from a flux polytope, polytope vertices
will be sampled with probability 0.  So what should we do? If we trust
our previous argument -- especially the fact that optimal flux
distributions, according to FCM, are elementary modes
\cite{wpht:14,murs:14} -- a uniform flux sampling might be
unrealistic, and we should rather sample polytope vertices. Bu to
account for unknown circumstances (e.g.~preemptive expression),
sampling the entire polytope may be a better strategy. \co{it depends
  on what we want: if we want to sample POTENTIALLY optimal {\flow}s, the
  interior of the polytope can be discarded; if we sample uniformly to
  approximate a Boltzmann-sampling with flux cost as energy, this is
  OK}
  
  \co{Heuristic criteria for choosing between flux profiles exist, but
    they rely on details of kinetics and enzyme {{\investment}}
    function, which require additional assumptions like the assumption
    of uniform {{\enzymeinvestment}}s, or estimated flux costs.}  \co{The
    practical procedure involves a choice of fluxes PRIOR to the
    choice of economic potentials.}  \co{In any case, theory can help
    us see what follows from our (potentially limited or wrong)
    optimality assumptions.}
\co{4: PRACTICAL CHOICE: PICKING A REPRESENTATIVE, NON-SPARSE
  SOLUTION. Still, sampling or picking a single solution would be suggested by a
  principle of insufficient reason: without any additional knowledge,
  it would be implausible to pick one of the edges by chance. However,
  in doing so, we should keep in mind that the solution we pick does
  not only have zero probability, but that it is also worse than the
  best solution on the polytope surface.}

\co{WO? RUNTER ZU abschnitt ueber PFK/FBAsse (``Beispielmodelle'')?
  EXAMPLE: Economic balance in overflow metabolism (may rather in CBA labour?)

\begin{figure*}[t!]
 \begin{center}
 \includegraphics[width=8cm]{\psfilesfluxes/example_overflow_balance.eps}
 \caption{\co{WRITE ME}}
 \label{fig:overflowBalance}
 \end{center}
\end{figure*}

  [WRITE ME!]
  
  Transport - Glycolysis (2 ATP) - Overflow bzw TCA (18 ATP) two
  There are two elementary {\flow}s (fermentation + respiration)

  Consider mixed {\flow}s:

  $\vv = \sigma \,\vv_{\rm F} + (1-\sigma)\, \vv_{\rm R}$

  $\Delta w = 2\, \sigma \,w_{\rm ATP} + 20\, (1-\sigma)\, w_{\rm ATP} = (20-18\,\sigma) w_{\rm ATP}$

  Total flux benefit:

  $\Delta w \cdot v = z = z_{\rm trans} + \sigma \,y_{\rm F} + (1-\sigma)\, y_{\rm R}$

  \begin{eqnarray}
    \Delta w &=& a_{\rm trans} + \sigma \,a_{\rm F} + (1-\sigma)\, a_{\rm R} \\
             &\ge& a_{\rm trans} + \sigma \,a^{\rm min}_{\rm F} + (1-\sigma)\, a^{\rm min}_{\rm R}\\
             &=& a_{\rm trans} + a^{\rm min}_{\rm R} + \sigma\, (a^{\rm min}_{\rm F}-a^{\rm min}_{\rm R})
  \end{eqnarray}
  So altogether
  \begin{eqnarray}
    20 w_{\rm ATP}- a_{\rm trans} - a^{\rm min}_{\rm R} &=& \sigma \,(18 \,w_{\rm ATP} + a^{\rm min}_{\rm F}-a^{\rm min}_{\rm R}) \\
    \Rightarrow 
    \sigma  &=& \frac{20 w_{\rm ATP}- a_{\rm trans} - a^{\rm min}_{\rm R}}{(18 \,w_{\rm ATP} + a^{\rm min}_{\rm F}-a^{\rm min}_{\rm R})}                                                           
  \end{eqnarray}
  Critical $a_{\rm trans} = 20 \,w_{\rm ATP} - a^{\rm min}_{\rm R}$. Above this value, $\sigma =0$ and
  $20 \,w_{\rm ATP} = a_{\rm trans} + a_{\rm R}$, i.e. the ATP value increases.

}

\section{Algorithms for economic flux balance analysis}
\label{sec:algorithmsflux}

\subsection{How to calculate economical flux modes and economic potentials}

\coout{\ \\Computing economical fluxes and economic potentials in a
  network} According to the benefit principle, active enzymes in
enzyme-optimal states must have positive influences on the
{\metabolicobjective}.  This implies that the {\flow} $\vv$ must satisfy the
{\fluxbenefitbalance} Eq.~(\ref{eq:reactionbalanceeq}),
$[\Deltar w+ \bvdirs]v = \zcostgenerics$ with internal economic potentials
$\winti$ and positive {{\enzymeinvestment}}s $\zcostgenerics_{l}$.  To employ this
principle in FBA, we treat the economic potentials as variables and
impose the {\fluxbenefitbalance} as a constraint.  Given the flux
{\gain}s $\bvtotl$, we can then determine the stationary fluxes
$v_{l}$, chemical potentials $\mu_{i}$, and economical potentials
$\wintm$ by requiring stationarity, thermodynamic sign constraints, and
the {\fluxbenefitbalance} equation. In practice, solutions can be
found by mixed-integer linear programming. But this may be difficult,
and we can also compute the variables step by step:

\begin{enumerate}[leftmargin=5mm]
\item \textbf{Flux pattern}
  First, we determine a {\flow} with thermodynamically and
  economically feasible flux directions. Such {\flow}s can be obtained by
  flux cost minimisation. By running FCM with different choices of flux cost
  weights, we obtain {\flow}s with different {\fluxpattern}s.
  Alternatively, we can start from some uneconomical metabolic {\flow} and
  remove all flux cycles and {\nonbeneficial} modes (see
  \ref{sec:removefutilecycles}).
\item \textbf{FLow} Based on our feasible flux pattern, we can
  construct various {\flow}s with this \fluxpattern and with more
  realistic flux magnitudes. Such {\flow}s can be obtained by FBA or by
  flux sampling. \co{andere tricks?}
\item \textbf{Economic potentials and {{\enzymeinvestment}}s} Given the flux
  directions, we next determine chemical and economic potentials.  In
  the calculation, we use the {\fluxbenefitbalance} as a linear
  constraint and determine the economic potentials by linear
  optimisation or by sampling; the {{\enzymeinvestment}}s $\zcostgenerics_{l}$ follow
  automatically from the {\fluxbenefitbalance}.  The resulting fluxes
  and economic potentials will be formally feasible, but possibly
  unrealistic (i.e.~very different from the fluxes and economic
  potentials that would be obtained from realistic kinetic models).
  For example, if we sample the economic potentials, the resulting
  {\enzymeinvestment}s may imply very large {{\investment}}s in unimportant
  enzymes. To obtain realistic potentials, we may account for known
  enzyme properties such as molecular weights or catalytic constants,
  use other data, e.g. known or guessed fluxes and enzyme levels, or
  employ some heuristic assumptions (see sections
  \ref{sec:princdistribinvestment} and
  \ref{sec:potentaislfromenzymepar}).
\item \textbf{Constructing other solutions by varying a given
    solution} Once we have found a solution, we may vary it to
  generate other, more realistic solutions.  Starting from fluxes
  $\vv$ and economic potentials $\wint$, we may keep the economic
  potentials $\winti$ fixed, vary individual fluxes (where the fluxes
  need to remain stationary and flux signs are fixed), and vary all
  {{\enzymeinvestment}}s proportionally. Alternatively, we may fix the
  fluxes and vary the {\fluxvalue}s $\Deltar \wtotl + \bvdirl$ and
  costs $\zcostgenerics_{l}$ proportionally. Finally, in models with moiety
  conservation (e.g.~[ATP] + [ADP] = const), we may vary the economic
  potentials by adding an arbitrary conserved moiety vector
  $\mathfrak{g}$ (satisfying $\mathfrak{g}\trans \,\Ntot=0$) to
  $\wtot$. The potential differences $\Deltar \wtotl$
  (e.g.~$w_{\Deltar \rm ATP} = w_{\rm ATP}-w_{\rm ADP}-w_{\rm
    phosphate}$), {{\enzymeinvestment}}s, and enzyme benefits will not be
  affected by this.  Starting from a solution ($\vv, \wint, \hudot$)
  and varying it in these ways, we obtain an ensemble of possible
  solutions, or we can construct solutions that comply with other
  knowledge or data.
\end{enumerate}

\subsection{How to check flux modes for being economical}
\label{sec:appcriteria} 

\myparagraph{\ \\Criterion for economical metabolic {\flow}s} A {\flow}
$\vv$ is called economical if it satisfies the {\summationcondition}
Eq.~(\ref{eq:fitnessbalance2}).  Eq.~(\ref{eq:fitnessbalance2})
applies only to {\flow}s in which all reactions are active. By
definition, a {\flow} with inactive reactions economical if the same
flow, with all inactive reactions omitted, is
economical\footnote{Inactive reactions can be ignored and be removed
  from the model. To justify their vanishing fluxes, we can always
  assume large {{\enzymeprice}}s in the underlying kinetic
  model.}. Economical {\flow}s must satisfy the flux variation criterion
\cite{lieb:14a}, which compares an economical {\flow} $\vv$ to a test
mode $\modevector$ (i.e.~a stationary {\flow} on the active region of
$\vv$). For an economical {\flow}, the following holds: (i) If
$\modevector$ is beneficial ($\bvtot\cdot \modevector>0$), then $\vv$
and $\modevector$ must share some active reaction with the same flux
directions.  (ii) If $\modevector$ is {\wasteful}
($\bvtot\cdot \modevector<0$), then $\vv$ and $\modevector$ share some
reaction with the opposite flux directions. (iii) If $\modevector$ is
{\futile} ($\bvtot\cdot \modevector=0$), they must share both sorts
of reactions. This leads to the submode criterion: economical {\flow}s
must not contain any {\nonbeneficial} submodes\footnote{In a model with a
  production objective, this criterion shows that an economical flux
  profile is thermodynamically feasible: if there were an elementary flux
  cycle, indicating thermodynamic infeasibility, the {\flow} would be
  uneconomical.}. To apply this criterion, we only need to consider
elementary test modes. The submode criterion implies that economical
metabolic {\flow}s $\vv$ are beneficial (i.e.~have a positive total flux
benefit $\bvtot\cdot\,\vv$). To see this, we insert $\kv=\vv$ into the
{\summationcondition} Eq.~(\ref{eq:fitnessbalance2}) and obtain the
equality $\sum_{l} \zcostgenerics_{l} = \bvtot\cdot \vv$. Since the
{{\enzymeinvestment}}s $\zcostgenerics_{l}$ are positive, the benefit must also be
positive.

\myparagraph{Practical tests for economical {\flow}s} Constructing
feasible metabolic {\flow}s can be difficult because the thermodynamic and
economic flux constraints are nonlinear. The resulting mixed-integer
linear problems are numerically much harder than linear FBA. However,
checking a given {\flow} $\vv$ is relatively easy: it amounts to solving
linear satisfiability problems. There are several possibilities:
\begin{enumerate}[leftmargin=5mm]
\item \textbf{{\Summationcondition}.}  To satisfy the variation
  condition (\ref{eq:fitnessbalance2}), there must be {\fluxburden}s
  $\hvl$, with the same signs as the fluxes $\v_{l}$, satisfying
\begin{eqnarray}
 {\Kint}\trans \hvv &=& {\Kint}\trans \bvtot \nonumber \\
 \label{eq:signvectorcondition1}
 \diag(\vv)\, \hvv &>&0.
\end{eqnarray}
${\Kint}$ is a right-kernel matrix of $\Nint$ and its columns span the
space of stationary flux distributions.  The inequality ensures that
$\vv$ and $\hvv$ have the same sign patterns.

\item \textbf{{\Fluxbenefitbalance}: check the existence of
  consistent economic potentials.} An {\complete} {\flow} $\vv$ is
  economical if and only if it satisfies the benefit principle
\begin{eqnarray}
 \label{eq:signvectorcondition12}
 \diag(\vv)\, ({\Nint}\trans \wint + \bvtot) &>&0,
\end{eqnarray}
 with a  vector $\wint$ to be determined.  For  a practical test this, we search for 
 a difference vector $\Deltar \wint$ satisfying 
\begin{eqnarray}
 \label{eq:signvectorcondition13}
 \diag(\vv)\, (\Deltar \wint + \bvtot) &>&0 \nonumber\\
 {\Kint}\trans \,\Deltar \wint &=& 0.
\end{eqnarray}
The second line is a Wegscheider condition for $\Deltar \wint$,
ensuring that $\Deltar \wint = {\Nint}\trans \wint$ with some vector
$\wint$ \cite{wegs:02,scsc:89}.  Even if $\bvtot$ is not
known, we can constrain it by inequalities of the form
$\Qmat\, \bpsi > \qv$, which puts
 constraints on the flux directions. In this case, to show that a
flow $\vv$ is economical, we need to find a vector
${\bpsi \choose \hudot}$ such that
\begin{eqnarray}
 \label{eq:vbaconstraint2}
 {\Kint}\trans \left({\Next}\trans,\,-\diag(\vv)\inv\right) { \bpsi\choose \hudot} &=& 0 \nonumber\\
 \begin{pmatrix} \Qmat &0 \\0& \Imat\end{pmatrix} { \bpsi\choose \hudot} &>& {\qv \choose 0}.
\end{eqnarray}
\end{enumerate}
The criteria (\ref{eq:signvectorcondition1}) and
(\ref{eq:vbaconstraint2}) do not concern only  {\flow}s with inactive
reactions. Thus, to use this criterion, all inactive reactions must
first be removed from the model. Eqs (\ref{eq:signvectorcondition12})
and (\ref{eq:signvectorcondition13}), in contrast, apply directly to
the active reactions, while inactive reactions can be ignored (and 
their vanishing fluxes can be justified by assuming high
{{\enzymeprice}}s).

\subsection{How to eliminate thermodynamically or infeasible submodes} 
\label{sec:removefutilecycles} 

If no consistent chemical (or economic) potentials canbe found for a
given {\flow}, we know that this {\flow} is thermodynamically (or economically)
infeasible. But how can we localise the problem, i.e.~how can we
detect the problematic reactions or cycles, and how can we know which
fluxes need to be set to zero to obtain a feasible flux distribution?
Cyclic submodes (which violate thermodynamic laws) can be detected and
removed with the help of elementary flux modes.  Futile submodes
(which make a {\flow} uneconomical) can be treated similarly.  For
medium-sized networks, the elementary cyclic modes can be enumerated
by \emph{efmtool} \cite{efmtool} and be collected as columns in a
matrix $\Cmat$. Let $\vv$ be the {\flow} in which flux cycles should be
found and removed.  First, we reorient all reactions to avoid negative
fluxes.  Depending on the feasibility criterion we are interested in
(weak or strong thermodynamic feasibility, see SI
\ref{sec:metabolicmodels}, or economic feasibility), there are
different algorithms (see Figure \ref{fig:corrections}):

\begin{enumerate}[leftmargin=5mm]
\item \textbf{Respecting the strong thermodynamic condition} The strong thermodynamic
  flux condition states that non-zero driving forces cause non-zero
  fluxes in the same direction. To comply with such a condition, $\vv$
  must be sign-orthogonal on all cyclic {\flow}s $\modevectorcyc$
  (see section \ref{sec:metabolicmodels}).  As a test, we enumerate
  all elementary cyclic {\flow}s $\modevectorcyc$ (the columns of
  $\Cmat$, not limited to the support of $\vv$) that are conformal
  with $\vv$ (i.e.~that have positive or vanishing, but not negative
  fluxes on the support of $\vv$). Any such {\flow} indicates a
  constraint violation. To correct $\vv$, we compute the mean ratio
  $\xi = \langle \frac{v_l}{k_l} \rangle_{l \in
    \mbox{supp}(\vv,\modevectorcyc)}$ and replace $\vv$ by
  $\vv' = \vv - \xi\,\modevectorcyc$. The corrected {\flow} $\vv'$
  is sign-orthogonal\footnote{The proof is simple. If all ratios
    $v_l/k_l$ on the overlap of $\vv$ and $\modevectorcyc$ are
    identical, the corresponding elements are eliminated in $\vv$ and
    there remain no non-zero elements common to $\vv'$ and
    $\modevectorcyc$.  Otherwise, some of the $\vv'$ values on
    the remaining overlap are positive and others are negative. In
    both cases, $\vv'$ and $\modevectorcyc$ are
    sign-orthogonal.} on $\modevectorcyc$.
\item \textbf{Respecting the weak thermodynamic condition} The weak
  thermodynamic condition resembles the strong thermodynamic flux condition,
  but it only holds for active reactions. It states that for any
  non-zero flux, there must be a thermodynamic force in the same
  direction. To comply with this condition, a {\flow} $\vv$ must be
  sign-orthogonal on all cyclic test modes $\modevectorcyc$
  (i.e.~on all columns of $\Cmat$ whose supports are within the
  support of $\vv$).  To test this, we enumerate all elementary cyclic
  test modes $\modevectorcyc$.  If we find one that is
  conformal with $\vv$, this shows that the constraint is violated. To
  repair the constraint violation, we compute
  $\xi = \mbox{min}_{l \in \mbox{supp}(\vv,\modevectorcyc)}
  v_l/k_l$ and define the corrected {\flow}
  $\vv' = \vv - \xi\,\modevectorcyc$, which is sign-orthogonal
  on $\modevectorcyc$. The proof is simple: our correction
  makes (at least) one of the fluxes in the cycle (defined by
  $\modevectorcyc$) vanish, but it does not revert any
  fluxes. Thus, $\vv'$ and $\modevectorcyc$ are
  sign-orthogonal.
\item \textbf{Respecting the economic condition} Non-beneficial
  submodes can be found and removed in a similar manner.  We use
  the same test as for the weak thermodynamic constraints, but considering
  {\futile} modes $\modevectorfut$ instead of cyclic modes
  $\modevectorcyc$ as test modes.  The number of elementary
  {\nonbeneficial} modes can be large, which makes the calculation more
  expensive.
\end{enumerate}

\textbf{Remarks:} (i) In all three cases, we only need to check
\emph{elementary modes}. If a constraint is violated by a
non-elementary mode, it will also be violated by some elementary
mode. In contrast, if there are no constraint violations by any
elementary modes, there are also no constraint violations by any
non-elementary modes.  (ii) In all three cases, the correction
procedure can be run iteratively until no constraint violations
remain.  In the cases 2 and 3 (weak thermodynamic condition and economic
condition), this procedure removes all constraint violations (because
in every step, fluxes are switched off, while no fluxes change their
directions). In the first case (strong thermodynamic constraint), a
correction step may change some flux directions, and there is no proof
that the iterative procedure converges to a feasible flux profile.

\begin{figure*}[t!]
 \begin{center}
 \includegraphics[width=16cm]{\psfilesfluxes/corrections.eps}
 \caption{Infeasible patterns in metabolic {\flow}s can be detected and
   removed by inspecting elementary flux modes. We consider three
   types of constraint. (a) Strong thermodynamic constraints. (b) Weak
   thermodynamic constraints. (c) Economic constraints. }
 \label{fig:corrections}
 \end{center}
\end{figure*}

\coout{What about
  other conditions, for instance, more rows in Naug? Mention this in
  paper: everal objectives: adding more neutrality requirements =
  fewer elementary modes = helps to check for fluxes that optimise
  NONE of the alternative objectives?}

\subsection{Algebraic constraints on  {\fluxburden}s}
\label{sec:SIAlgConstraintFluxBurden}

\myparagraph{\ \\The {\fluxburden} vector $\hvv$ in an optimal state is
  orthogonal on all {\futile} flux modes}
We consider a model with a flux objective (i.e.~no cost effect of
metabolite concentrations). If $\vv$ is an economical {\flow} and $\vv_{\rm fut}$
is a {\futile} flux mode, the {\summationcondition} implies the equality 
\begin{eqnarray}
 \vv_{\rm fut}  \odots (\hudot \oslashs \vv) = 0.
\end{eqnarray}
This means that the flux {{\price} vector $\hvv = \hudot \oslashs \vv$ in
  an optimal state is orthogonal on all futile flux modes
  $\vv_{\rm fut}$. This holds, in particular, for all {\flow}s
  $\vv_{\rm fut} = \kv^{(1)}-\kv^{(2)}$, where $\kv^{(1)}$ and $\kv^{(2)}$
  are {\flow}s with identical flux benefit.

\paragraph{The {\fluxburden} vector $\hvv$ lies in the image space of $\Nobj\trans$}
Let $\Kobj$ be a maximal right-kernel matrix of
$\Nobj = {\bvtot\trans \choose \Nint }$, satisfying
$\Nobj\, \Kobj = 0$. Then any {\futile} flux vector $\vv_{\rm fut}$
can be written as a linear combination of the columns of $\Kobj$, and
the {\summationcondition} (for models with a flux objective) can be
written
\begin{eqnarray}
  \label{eq:loop5}
  \Kobj\trans (\hudot \oslashs \vv) = 0.
\end{eqnarray}
This means that  the {\fluxburden} vector $\hvv = \hudot \oslashs \vv$ must be a
linear combination of the columns of $\Nobj\trans$.

\subsection{How to compute economic potentials based on heuristic
  assumptions}
\label{sec:princdistribinvestment}

In the \fluxbenefitbalance \ref{eq:reactionbalanceeq}, a given
metabolic {\flow} $\vv$ constrains the economic potentials $\winti$, but it 
does not determine them precisely. This means that there is some freedom of
choice.  How can we choose plausible economic potentials,
i.e.~potentials that we expect to find in  realistic kinetic
models?  We assume that $\vv$ is economical, i.e.~that a solution for
$\wint$ exists.  To obtain a realistic solution, we can make heuristic
assumptions about the enzyme costs $\zcostgenerics_{l}$. We consider two
possibilities. We either assume that all enzymes have similar
costs (``postulate of uniform {{\enzymeinvestment}}s''), or assume some
predefined set of cost values and try to approximate it as closely as
possible with our economic potentials.  In networks with conserved
moieties, there will be some gauge freedom in choosing $\wint$
(right-kernel vectors of ${\Nint}\trans$ can be freely added); to
obtain a unique solution, an additional regularisation condition can 
be applied (e.g.~minimising the norm $||\wint||^2$).

\begin{itemize}[leftmargin=5mm]
\item \textbf{Economic potentials that correspond to uniform
    {{\enzymeinvestment}}s.}  Given an {\complete} economical metabolic {\flow}
  $\vv$ and a {\fluxgain} vector $\bvtot$, our aim is to find
  internal economic potentials $\wint$ and {{\enzymeinvestment}}s $\hudot$
  that satisfy the {\fluxbenefitbalance} and that agree with our
  heuristic assumptions.  Summing over all {\fluxbenefitbalance}s (and
  assuming that all reactions are enzyme-catalysed), we obtain the
  equality
 \begin{eqnarray}
 \label{eq:balancedinvestments1}
 \sum_{l} \zcostgenerics_{l} = \sum_{l} \partial \hul\, \ul = \sum_{l} [\Deltar \wintl + \bvtotl]\,v_{l} = \bvtot\cdot \,\vv.
 \end{eqnarray}
 To satisfy this equation by a choice of internal economic potentials
 $\wint$, we apply a assumption: all enzymes should have similar
 {\costshade}s. For deriving the formula, we first consider a
 simplified case.  If the {{\enzymeinvestment}}s could be freely varied, we
 could realise our assumption by minimising $\sum_{l} (\zcostgenerics_{l})^{2}$,
 the sum of squared {{\enzymeinvestment}}s, under the constraint
 $\sum_{l} \zcostgenerics_{l} = \bvtot\cdot \,\vv$. With a Lagrange multiplier
 $\alpha$, we can formulate this as
 \begin{eqnarray}
 \label{eq:balancedinvestments00}
 \mbox{Minimise}\; && \sum (\zcostgenerics_{l})^{2} - \alpha (\sum_{l} \zcostgenerics_{l} - \bvtot\cdot \,\vv).
 \end{eqnarray}
 The solution $\zcostgenerics_{l}= -\alpha/2 = \const$ shows that all
 {{\enzymeinvestment}}s are equal just as required. However, we cannot
 assume that the enzyme costs can be freely varied, because they
 depend on the economic potentials as
 $y_l = v_{l}\, [({\Nint}\trans\, \wint)_{l} + \bvtotl]$. Instead we
 use the internal economic potentials as free variables and obtain
 the variational principle
 \begin{eqnarray}
 \label{eq:balancedinvestments3}
 \mbox{Minimise}\; &&
 \sum (\zcostgenerics_{l})^{2} 
 = \sum_{l} \left(v_{l}\, [({\Nint}\trans\, \wint)_{l} + \bvtotl]\right)^{2}\qquad \mbox{w.r.t.}\quad \wint,
 \end{eqnarray}
where the {{\enzymeinvestment}}s must either be positive or
larger than some positive minimal value $\zcostgenerics_{l}^{\rm min}$:
 \begin{eqnarray}
 \label{eq:balancedinvestments4}
 \zcostgenerics_{l}^{\rm min} \le \zcostgenerics_{l} = v_{l} [\Deltar \wintl + \bvtotl].
 \end{eqnarray}
Altogether, we  obtain the quadratic optimality problem for $\wint$ 
 \begin{eqnarray}
 \label{eq:balancedinvestments4Opt}
 \mbox{Minimise}\; && {\wint}\trans\, \Nint\, \diag(\vv)^{2} {\Nint}\trans\, \wint
 + 2\, {\wint}\trans\, \Nint\, \diag(\vv)^{2}\,\bvtot \quad \mbox{w.r.t}\; \wint \nonumber \\
\mbox{subject to}
 &&\hudotmin \cdot {{\bf 1}} - \diag(\vv)\, \bvtot \le \diag(\vv)\,{\Nint}\trans \wint,
 \end{eqnarray}
 where ${{\bf 1}} = (1, 1, ..)\trans$.  \coout{ \footnote{ \co{Without
       the constraints, the solution would read
   \begin{eqnarray}
 \label{eq:balancedinvestments4a}
 \wint = - \left(\Nint\, \diag(\vv)^{2}\, \Nint\right)\inv \Nint\, \diag(\vv)^{2}\, \bvtot.
 \end{eqnarray}
 if the matrix $\Nint\, \diag(\vv)^{2} {\Nint}\trans$ is
 invertible. If this is not the case, then to pick a specific
 solution, the matrix inverse can be replaced by the
 pseudo-inverse.}}.}  In models with moiety conservation, the matrix
$\Nint\, \diag(\vv)^{2} {\Nint}\trans$ is not invertible, so the
solution will not be unique.  For a unique solution, we can add a
regularisation term, e.g.~$\beta ||{\wint}||^{2}$ with a small
prefactor $\beta$. The calculation works only for {\complete} flux
profiles; inactive reactions must be omitted from the model.

\item \textbf{Economic potentials that correspond ro given enzyme
    costs or {\fluxburden}s.} As another heuristics, we may fit the
  economic potentials to given {{\enzymeinvestment}}s $\zcostgenerics_{l}^{\rm
    data}$. Given the predefined fluxes and {\fluxgain}s, we first
  scale the presumable {\enzymeinvestment}s $\zcostgenerics_{l}^{\rm data}$ to satisfy
  the sum rule $\sum_{l} \zcostgenerics_{l}^{\rm data} = \bvtot\cdot \,\vv$
  (Eq.~(\ref{eq:balancedinvestments1})). Then, to compute the economic
  potentials we postulate that the ratios $\zcostgenerics_{l}/\zcostgenerics_{l}^{\rm data}$
  must be similar for all enzymes. We implement this by the principle
  of known {\enzymeinvestment}s
 \begin{eqnarray}
 \label{eq:balancedinvestments5}
\mbox{Minimise}\;
 \sum \frac{(\zcostgenerics_{l})^{2}}{\zcostgenerics_{l}^{\rm data}} \qquad \mbox{subject to}\quad\sum \zcostgenerics_{l} = \sum_{l} \zcostgenerics_{l}^{\rm data}.
 \end{eqnarray}
 We obtain a slightly different quadratic
 optimality problem for $\wint$, with the same constraints:
\begin{eqnarray}
 \label{eq:balancedinvestments6}
\mbox{Minimise}\;
&& {\wint}\trans\, \Nint\, \diag(\vv)^{2}\, \diag({\hudot}^{\rm data})\inv {\Nint}\trans\, \wint
 + 2\, {\wint}\trans\, \Nint\, \diag(\vv)^{2}\,\diag({\hudot}^{\rm data})\inv\,\bvtot \nonumber \\
\mbox{subject to}
 &&\hudotmin \cdot {{\bf 1}} - \diag(\vv)\, \bvtot \le \diag(\vv)\,{\Nint}\trans \wint.
\end{eqnarray}
Again, regularisation may be used to obtain unique solutions in models
with moiety conservation.  By inserting our result $\wint$ into the
{\fluxbenefitbalance}, we obtain the {{\enzymeinvestment}}s $\hudot$, which
approximate the predefined {{\enzymeinvestment}}s ${\hudot}^{\rm data}$.  This
principle can be applied in various ways: (i) we can start from
presumable {\enzymeinvestment}s obtained from protein sizes and proteomics
data (see section \ref{sec:potentaislfromenzymepar}); (ii) we can
require uniform {\enzymeinvestment}s across all enzymes (and reobtain our
previous heuristics); (iii) we can assume given or uniform flux
{\price}s $\hvl^{\rm data}$ (estimated from protein properties alone;
see \ref{sec:potentaislfromenzymepar}) and set
$\zcostgenerics_{l}^{\rm data} = \hvl^{\rm data}\,v_l$; or (iv) the algorithm can
be applied to randomly sampled {{\enzymeinvestment}}s ${\hudot}^{\rm data}$ to
obtain an ensemble of enzyme-balanced models.

\end{itemize}

\subsection{How to estimate enzyme costs from enzyme molecule properties}
\label{sec:potentaislfromenzymepar}

\myparagraph{\ \\Estimation of {{\enzymeinvestment}}s} How can we estimate
the {{\enzymeinvestment}}s $\zcostgenerics_{l}=\hul\,\ul$ from measured metabolic flux and
proteome data?  We assume that the costs are proportional to
measured enzyme levels $e^{\rm data}_{l}$. For the {{\enzymeprice}}s, we
assume a proportionality
\begin{eqnarray}
\label{eq:enzymeparametersandforce1}
\hul \sim L_{l}\,(\lambda + \enzdegrate_{l})
\end{eqnarray}
with enzyme sizes $L$ (number of amino acids), cell growth rate
$\lambda$, and enzyme degradation rates $\enzdegrate_l$
\cite{lieb:14a}.  For the absolute scaling, we can rescale the
{\enzymeinvestment}s by a prefactor
$\frac{\bvtot\cdot \vv}{\sum_{l}\, \zcostgenerics_{l}^{\rm data}}$. The rescaled
{\enzymeinvestment}s will sum to the total flux benefit $\bvtot\cdot \vv$.

\myparagraph{Estimation of {\fluxvalue}s from enzyme parameters} In
kinetic models the economic potentials $\wtoti$ and {{\enzymeprice}}s
$\hul$ are related to enzyme kinetics and, in particular, to the
catalytic constants $\kcat$.  How can we use known catalytic constants
to estimate the economic potentials?  In enzyme-optimal states, the
equation $\Deltar \wtot + \bvdir = \hvv$ must be satisfied. The flux
{\burden}s $\hvs = \hus\,u/v$ are state-dependent and thus variable,
but in any case they need to satisfy some constraints.  A reaction
rate is given by $\rate(\cv)=u\,\ratelaw(\cv)$ with an enzyme
efficiency $\ratelaw$ in the range
$-k^{\rm cat-} \le \ratelaw \le k^{\rm cat}$. If we assume a positive
flux, the flux can be approximated by
\begin{eqnarray}
\label{eq:enzymeparametersandforce2}
\hvs = \frac{\hus}{\ratelaw} = \alpha_{\rm scale} \frac{L\,(\lambda + \enzdegrate)}{\ratelaw}
\ge \alpha_{\rm scale} \frac{L\,(\lambda + \enzdegrate)}{k^{\rm cat}\,(1-\e^{\Deltar G/RT})}.
\ge \alpha_{\rm scale} \frac{L\,(\lambda + \enzdegrate)}{k^{\rm cat}},
\end{eqnarray}
where $\lambda + \enzdegrate$ is the proteins's effective degradation
constant, $L$ is its amino acid chain length, and $\alpha_{\rm scale}$ is a
scaling factor. To determine $\alpha_{\rm scale}$, we set the sum
$\sum_{l} \hvl\,v_{l}$ equal to the total {{\enzymeinvestment}}, $y_{\rm tot} =
\sum_l \hvl \, v_l = \alpha_{\rm scale} \sum_l \frac{L\,(\lambda +
  \kappa)\,v_l}{k^{\rm cat}}$, and obtain $\alpha_{\rm scale} = \frac{y_{\rm
    tot}}{\sum_l \frac{L\,(\lambda + \enzdegrate)\,v_l}{k^{\rm cat}}}$.
When an enzyme operates at its maximal  speed, its specific rate is given by
$\ratelaw_{l} = k^{\rm cat}_{+}$ (or, in the case of negative fluxes,
$\ratelaw_{l} = -k^{\rm cat}_{-}$).  In VBA, the expressions in
Eq.~(\ref{eq:enzymeparametersandforce2}) can be used to estimate or
delimit the   {\fluxburden}s $\hvl=\zcostgenerics_{l}/v_{l}$ or
the {\fluxvalue}s $\Deltar \wtotl + \bvdirl$.

 \myparagraph{Correction of estimated {\fluxburden} based on
   {\summationconnectivitycondition}} To estimate $\hvv$ by equation
 (\ref{eq:enzymeparametersandforce2}), we need to know the flux directions, but
 not the quantitative fluxes. If the fluxes $v_{l}$,
 enzyme levels $\ul$, and enzyme {\price}s $\hul$ are known, we can determine
 the {\fluxburden}s $\hvl = \hul \frac{\ul}{v_{l}}$. However, the data values (fluxes or enzyme levels) are typically imprecise,. In this case,
 additional constraints on $\hvv$ can be used to improve
 our estimates. To satisfy  the flux benefit balance, {\fluxburden}s
 $\hvl$ and {\fluxgain}s $\bvtotl$ must satisfy the condition
\begin{eqnarray}
\hvv - \bvtot = {\Nint}\trans {\wint}\trans \in \mbox{Span}({\Nint}\trans).
\end{eqnarray}
Measured or estimated {\fluxburden}s are likely to  violate this
equation. To correct them, we compute  the
left-hand side and project it onto the hyperplane spanned by the columns of
${\Nint}\trans$.  From the {\fluxgain} condition
Eq.~(\ref{eq:fitnessbalance2}), we obtain similar constraints: the
vector $\hvv$ must be orthogonal on all {\futile} flux test modes
$\kv_{\rm fut}$. 
If we define $\Nobj = {{\bvtot}\trans \choose \Nint}$, and
its kernel matrix $\Kobj$ satisfying
${{\bvtot}\trans \choose \Nint} \,\Kobj=0$, then ${\hvv}$ must satisfy
${\hvv}\trans\,\Kobj=0$ and must thus be a linear combination of the
columns of $\Nobj\trans$.  In models with a pure concentration
objective (i.e.~$\bvtot=0$), the vector $\hvv$ must be orthogonal on
\emph{all} stationary {\flow}s, i.e.~it must be a linear combination of
the columns of ${\Nint}\trans$.  Finally, the {\fluxburden}s must
satisfy the {\connectivitycondition} \cite{lieb:14a}
\begin{eqnarray}
\label{eq:constraintforfluxprices}
(\Eunint\,\Lmat)\trans\,\hvv = -\Lmat\trans\,\bc
\end{eqnarray}
with the unscaled elasticity matrix $\Eunint$ and the link matrix
$\Lmat$.  In contrast, in models with a pure flux objective
(i.e.~$\bc = 0$), the {\fluxburden} vector $\hvv$ must be orthogonal
on all columns of $\Eunint\, \Lmat$. In linear pathways, this yields a
direct  relationship between elasticities and flux
{\burden}s in the same reactions.
From the estimated {\fluxburden}s $\hvl^{\rm est}$, we can
determine corrected {\fluxburden}s $\hvl$ by a least-squares
regression (requiring $\hvl \stackrel{!}{\approx} \hvl^{\rm est}$) under the
constraints given by Eq.~(\ref{eq:constraintforfluxprices})).

\myparagraph{Conversion of {\fluxvalue}s into economic potentials}
If the {\fluxvalue}s $\gvtotl$ in a model are known, they will
constrain the economic potentials $\winti$. To determine a single
solution, we can pick one of them by minimising the Euclidean norm
$||\winti||$ under the constraint
$\gvtotl = \Deltar \wtotl + \bvdirl$.  If also the fluxes are given,
there is a second possibility: we may translate $\gvtotl$ into the
{{\enzymeinvestment}s} ${\zcostgenerics}_{l} = \gvtotl \,v_{l}$ and proceed as
described in section \ref{sec:princdistribinvestment}.  If lower
bounds $\zcostgenerics^{\rm min}$ are known, we first need to check that the
constraint $\zcostgenerics_{l}> \zcostgenerics_{l}^{\rm min}$ is satisfied.

  \section{Fluxes and potentials in the PFK/FBPase cycle}

  \co{ist der abschnitt gut? dann ref in main text!} \todo{The
    possible fluxes in the PFK/FBP system are closely related to the
    chemical and economic potentials. The fact that PFK is only used
    for glycolysis and FBPase is only used for gluconeogenesis can be
    understood by combining thermodynamic and economic constraints.
    Since both reactions can theoretically run in forward or reverse
    direction or be shut off, we obtain nine possible sign
    combinations, two of which correspond to the typical fluxes in
    glycolysis (PFK foward/FBPase off) and glyconeogenesis (PFK
    off/FBPase forward). In fact, under relatively general
    assumptions, all other sign combinations can be ruled out by the
    thermodynamic and economic constraints. If we assume that the ATP
    has a higher chemical potential and a higher economic potential
    than ADP, three out of nine possible sign combinations can be
    excluded. And under physiological conditions, either PFK or FBPase
    is active (each in forward direction), or both are shut off.

To study this in more detail, we list all possible flux patterns and check
them for thermodynamic and economic feasibility.  We consider the
potentials of four metabolites ADP (plus inorganic phosphate; denoted
by A), ATP (plus water; denoted by B), as well as F6P (X) and FBP
(Y). We assume that under all physiological conditions, ADP (plus
phosphate) has a lower chemical potential $\mu_{A}<\mu_{B}$ than ATP
(plus water), and also a lower economic potential $w_{A}<w_{B}$. For
the chemical potentials of F6P and FBP, we also consider three
possible cases:
\begin{center}
 \begin{tabular}{llll}
   Case & Condition & (PFK/FBP) \\ 
   ($\alpha$) & $\mu_{X}<\mu_{Y}$                                      & infeasible & feasible \\ 
   ($\beta$)  & $\mu_{X}>\mu_{Y}$ but  $\mu_{X}+\mu_{A}<\mu_{Y}+\mu_{B}$  & infeasible & infeasible\\ 
   ($\gamma$) & $\mu_{X}+\mu_{A}<\mu_{Y}+\mu_{B}$                        & feasible & infeasible \\
 \end{tabular}
\end{center}
Likewise, for the economic potentials of F6P and FBP, we consider
three possible cases
\begin{center}
\begin{tabular}{llll}
  Case & Condition & PFK & FBPase \\ 
  (A) & $w_{X}<w_{Y}$                               & beneficial & \wasteful \\  
  (B) & $w_{X}>w_{Y}$, but $w_{X}+w_{A}<w_{Y}+w_{B}$   & beneficial & beneficial \\
  (C) & $w_{X}+w_{A}>w_{Y}+w_{B}$                     & \wasteful & beneficial
\end{tabular}
\end{center}
Altogether, we obtain nine possible scenrios.  Now we consider all
possible flux patterns and ask which of these scenarios they can be
realised. Note that vanishing fluxes are always allowed.

\begin{center}
\begin{tabular}{l|lll}
  & $v_{PFK} <0$        & $v_{PFK} =0$              & $v_{PFK} >0$            \\ 
\hline
  $v_{FBP}>0$  & case $\alpha$C       & cases $\alpha$B, $\alpha$C        & thermodynamically infeasible \\
  $v_{FBP}=0$  & cases $\alpha$C, $\beta$C  & always possible         & cases $\gamma$A, $\gamma$B     \\
  $v_{FBP}<0$  & economically infeasible & cases $\beta$A, $\gamma$A   &  case $\gamma$A       
\end{tabular}
\end{center}

Thus, the two cycle fluxes (PFK and FBPase both active in forward
direction, or both in reverse direction) are infeasible. The fluxes in
which both enzymes are active, either in glycolytic or gluconeogenic
direction are theoreticall feasible, but only under physiologically
unusual circumstances.

\begin{figure*}[h!]
  \begin{center}
\parbox{11cm}{\includegraphics[width=10.5cm]{\psfilesfluxes/pfk_example.eps}}
\parbox{5cm}{ 
%  \[ \Delta \mu_{\rm F} = \mu_{\rm FBP} - \mu_{\rm F6P}\]
%  \[ \Delta \wint_{\rm F} = \wint_{\rm FBP} - \wint_{\rm F6P}\]
%  \[ \Delta \mu_{\rm A} = \mu_{\rm ATP} - \mu_{\rm ADP}\]
%  \[ \Delta \wint_{\rm A} = \wint_{\rm ATP} - \wint_{\rm ADP} \]
% 
\coout{inaktive reaktionen in graphik gestrichelt zeigen}
 Energy and economic potential differences
 \begin{eqnarray*}
 \mu_{\rm PFK}    &=& \Delta \mu_{\rm F} - \Delta \mu_{\rm A} \\
   \wsymbol_{\rm PFK}    &=& \Delta   \wsymbol_{\rm F} - \Delta   \wsymbol_{\rm A} \\
 \mu_{\rm FBPase} &=& - \Delta \mu_{\rm F} \\
   \wsymbol_{\rm FBPase} &=& - \Delta   \wsymbol_{\rm }
 \end{eqnarray*}
}
\caption{\co{compare picture to table above. which one is better?}
  Thermodynamic and economic constraints in the PFK/FBPase loop.  (a)
  The enzymes phosphofructokinase (PFK) and fructose bisphosphatase
  (FBPase) can catalyse an ATP-consuming substrate cycle, but the flux
  cycle is usually suppressed in living cells.  (b) Feasible flux
  patterns.  According to VBA, the flux directions must agree
  with the differences between chemical potentials $\mu_{i}$ and
  economic potentials $\wsymbol_{i}$ along the reactions. The
  conversion from ATP to ADP requires a decrease
  $\Delta \mu_{\rm A} = \mu_{\rm ATP} - \mu_{\rm ADP}$ in chemical
  potential and amn increase
  $\Delta \wsymbol_{\rm A} = \wsymbol_{\rm ATP} - \wsymbol_{\rm ADP}$
  in economic potential.  In contrast, the differences
  $\Delta \mu_{\rm F} = \mu_{\rm FBP} - \mu_{\rm F6P}$ and
  $\Delta \wsymbol_{\rm F} = \wsymbol_{\rm FBP} - \wsymbol_{\rm F6P}$
  may depend on the situation. The table shows the feasible fluxes for
  different possible combinations. Feasible forward and reverse fluxes
  and mandatory zero fluxes are indicated by +, -, and 0 (where fluxes
  with a predefined sign are also allowed to vanish). If reactions
  have no direct {\fluxvalue}, and with physiologically plausible
  values for $\Delta \mu_{l}$ (centre column), the two enzymes cannot
  be active at the same time.}
    \label{fig:pfk_example}
  \end{center}
\end{figure*}

How would other flux prediction methods describe the PFK/FBPase
system?  FBA without sign constraints would yield another, must less
realistic result. it would predict the cycle to run in reverse
direction, converting inorganic phosphate into ATP, which is
thermodynamically impossible under physiological conditions.
Thermodynamic FBA, with realistic chemical potentials of ATP, ADP, and
inorganic phosphate, woudl avoid this cycle, but it would allow the
ATP-saving reverse use of FBPase for glycolysis; only if all chemical
potentials for both situations (glycolysis and gluconeogenesis) are
given, all wrong solutions are excluded, but this is trivial since the
flux directions would be predefined.}
